# Supplementary material for: Robust Safety-Critical Control for Dynamic Robotics
Source: arXiv:2005.07284 source file (2021-04-13)
Supplement: Supplementary file 1 [file appendix_QP_forms.tex]

\section{Derivation of QP based controllers}
\label{sec:appendix_QP_form}
In this Appendix, we will describe in details about how to formulate our proposed controller in a standard quadratic program formulation.
\subsection{CLF-QP}
\label{app:CLF-QP}
The CLF-QP controller with constraints \eqref{eq:RelaxedCLFQP} can be written as the following standard form of quadratic programs:

\HRule
\noindent \textbf{CLF-QP with Constraints}:
\begin{align}
\label{CLF_QP_form}
u^*(x)=	& \underset{u,\mu, \delta}{\argmin} & & \mu^T \mu + p \delta ^2\\
& \text{s.t.} & & A_{CLF}\begin{bmatrix}
\mu \\ \delta 
\end{bmatrix} \le b_{CLF}, \mytag{CLF}\\
&&& A_c(x) u \le b_c(x), \mytag{Constraints}\\
&&& u =u_{ff}(x) + (L_g L_f y(x))^{-1} \mu, \mytag{IO}
\end{align}
\HRule

where
\begin{align}
\label{def_AB_clf}
A_{CLF}=\begin{bmatrix}
L_{\bar g}V_\epsilon & -1
\end{bmatrix}, \quad
b_{CLF}=-L_{\bar f}V_\epsilon-\frac{c_3}{\epsilon}V_\epsilon.
\end{align}

\subsection{CBF-CLF-QP}
\label{app:CBF-CLF-QP}
The QP form of CBF-CLF-QP controller in \eqref{CBF_CLF_QP_constraints} is given by:
\HRule
\noindent \textbf{CBF-CLF-QP with Constraints}:
\begin{align}
u^*(x)=	& \underset{u,\mu,\delta}{\argmin} & & \mu^T \mu + p~\delta^2 \\
& \text{s.t.} & & A_{CLF}\begin{bmatrix}
\mu \\ \delta 
\end{bmatrix} \le b_{CLF},  \mytag{CLF} \\
& & & A_{CBF}~u \le b_{CBF}  \mytag{CBF} \\
&&& A_c(x) u \le b_c(x).\mytag{Constraints}\\
&&& u =u_{ff}(x) + (L_g L_f y(x))^{-1} \mu, \mytag{IO}
\end{align}
\HRule

where $A_{CLF},b_{CLF}$ are as defined in \eqref{def_AB_clf}, and
\begin{align}
A_{CBF}=L_gB, \quad b_{CBF}=\frac{\gamma}{B}-L_fB.
\end{align}

\subsection{Robust CLF-QP with constraints}
%QP form of \eqref{robust_CLF_QP_constraint}
\label{app:Robust CLF-QP}

%Note that the min-max inequality type optimization in \eqref{robust_CLF_QP_constraint} is actually a quadratic program.  To see this, 
Notice that the robust RES condition in \eqref{eq:robust_RES_cond} is affine in the control inputs $\mu$ and thus can be expressed as
\begin{equation}
\label{RESIneqUncertainty}
\max_{\substack{||\Delta_1||\le \Delta_1^{max} \\ ||\Delta_2||\le \Delta_2^{max} }} {\Psi}_{0}+{\Psi}_{1}\mu \le 0,
\end{equation}
where
\begin{align}
\label{TildePsi01Defns}
{\Psi}_{0}(\eta, \Delta_1)&:= L_{\bar{f}}V_\epsilon(\eta)%\etavar^T (F^T P_{\epsilon} + P_{\epsilon} F) \etavar + 2 \eta ^T P_{\epsilon} \Delta H 
+ \frac{c_3}{\epsilon}V_{\epsilon},\nonumber\\
{\Psi}_{1}(\eta, \Delta_2) &:= L_{\bar{g}}V_\epsilon(\eta),%2 \etavar^T P_{\epsilon} (G+ \Delta G).
\end{align}
with $L_{\bar{f}}V_\epsilon(\eta), L_{\bar{g}}V_\epsilon(\eta)$ as defined in \eqref{BarLfVandLgVUncertainty}.

The goal of the robust control design is then to find the control $\mu$ satisfying the RES condition \eqref{RESIneqUncertainty}, evaluated through the given bounds of uncertainty in \eqref{assump:BoundUncertainty}. However, our controller can only use the nominal model $\tilde{\bar f}, \tilde{\bar g}$ and not the true model $\bar f, \bar g$ (see Table \ref{tab:ModelTypes} for different types of models).  We thus define the Lie derivatives of $V$ with respect to the nominal model as
\begin{align}
L_{\tilde {\bar f}}V&=\etavar^T (F^T P_{\epsilon} + P_{\epsilon} F) \etavar, \\
L_{\tilde {\bar g}}V&=2 \etavar^T P_{\epsilon} G.
\end{align}
%Next, using the following virtual I-O linearization:
%\begin{align}
 %L_{\tilde{\bar g}}V \mu =: \mu_v,
%\end{align}
Then, from \eqref{BarLfVandLgVUncertainty}, we have
\begin{align}
\dot V &= L_{\bar f} V + L_{\bar g}V \mu \\
& = L_{\tilde{\bar f}}V 
	+ \underbrace{2\eta ^T P_{\epsilon} \begin{bmatrix}\textbf{0}\\\Delta_1\end{bmatrix} }_{\Delta_1^v} 
	+ \underbrace{L_{\tilde{\bar g}}V \mu}_{\mu_v} 
	+ \underbrace{L_{\tilde {\bar g}}\Delta_2 \mu }_{\Delta_2^v \mu_v}\\
& =L_{\tilde {\bar f}}V + \Delta_1^v + (1 + \Delta_2^v) \mu_v,
\end{align}
where we have defined the following new scalar variables: uncertainty $\Delta_1^v \in \mathbb{R}$, control input $\mu_v \in \mathbb{R}$, and uncertainty $\Delta_2^v\in \mathbb{R}$.
%\begin{align}
%L_{\tilde {\bar f}}V&=\etavar^T (F^T P_{\epsilon} + P_{\epsilon} F) \etavar, \\
%L_{\tilde {\bar g}}V&=2 \etavar^T P_{\epsilon} G,
%\end{align}
%are Lie derivatives of $V$ with respect to the nominal model of the I-O linearized system $\tilde{\bar f}, \tilde{\bar g}$ (see Table \ref{tab:ModelTypes} for different types of models on $f,g$). 
%
Since $\Delta_1^v$ is the model uncertainty on $L_{\bar f}V$ and $\Delta_2^v$ is the model uncertainty on the mapping of the control input $\mu_v$, we then can simply design robust CLF condition using the assumption on the bounds of $\Delta_1^v$ and $\Delta_2^v$. However, based on the model uncertainty analysis in \eqref{BarLfVandLgVUncertainty}, in order to consider the presence of the state $\eta$ in the model uncertainty, we will evaluate $\Delta_1^v$ using the following assumption:
\begin{align}
||\Delta_1^v|| & \le ||2 \eta ^T P_{\epsilon}  \begin{bmatrix}\mathbf{0} \\ \mathbf{1} \end{bmatrix}||\Delta_1^{max}.
\end{align}
This approach is frequently used in adaptive control to improve the performance of the adaptation law (see \cite{NgSr2014Adaptive_ACC}, \cite{L1:TransientPerformance:TAC08}). Since $\mu_v$ includes $L_{\bar g}V=2 \etavar^T P_{\epsilon} G$, and from \eqref{BarLfVandLgVUncertainty}, we therefore consider the following assumption for $\Delta_2^v$:
\begin{align}
||\Delta_2^v||\le \Delta_2^{max}
\end{align}

Therefore, the RES condition \eqref{RESIneqUncertainty} will hold if the following inequalities hold
\begin{align}
%\label{RESwithUncertaintyBoundCondition}
{\Psi}_{0}^{ max}+{\Psi}_{1}^p \mu \le 0, \nonumber \\
{\Psi}_{0}^{ max}+{\Psi}_{1}^n \mu \le 0,
\end{align}
where
\begin{align}
{\Psi}_{0}^{max}&= L_{\tilde{\bar f}}V+\frac{c_3}{\epsilon}V_{\epsilon}+||2 \eta ^T P_{\epsilon} \begin{bmatrix}\mathbf{0} \\ \mathbf{1} \end{bmatrix} ||\Delta_1^{max},\nonumber\\
{\Psi}_{1}^p& = L_{\tilde {\bar g}}V(1+\Delta_2^{max}),\nonumber\\
{\Psi}_{1}^n& =L_{\tilde {\bar g}}V(1-\Delta_2^{max}).
\end{align}
Thus the robust CLF-QP in \eqref{robust_CLF_QP} is then equivalent to the following optimization problem, which can clearly be seen as a QP:%We can then incorporate these inequalities into a new relaxed CLF-QP as follows:
%
%\HRule
%
%\noindent Robust CLF-QP:
\begin{align}
\label{cvxWithUncertainty}
\mu^* =& \underset{\mu}{\argmin} & & \mu^T \mu \\
& \text{s.t.} & & {\Psi}_{0}^{max}(\eta,\Delta_1^{max}) + {\Psi}_{1}^p(\eta,\Delta_2^{max})~\mu \le 0, \nonumber\\ & & & {\Psi}_{0}^{max}(\eta,\Delta_1^{max}) + {\Psi}_{1}^n(\eta,\Delta_2^{max})~\mu \le 0. \nonumber
\end{align}
Incorporating the above robust CLF constraint we have the following Robust CLF-QP with constraints:
\HRule
\noindent \textbf{Robust CLF-QP with Constraints}:
\begin{align}
\label{Robust_CBF_CLF_QP_form}
u^*(x)=& \underset{u,\mu, \delta_1, \delta_2}{\argmin} & & \mu^T \mu + p_1 \delta_1 ^2 + p_2 \delta_2^2\\
& \text{s.t.} & & {\Psi}_{0}^{max}(\eta,\Delta_1^{max}) + {\Psi}_{1}^p(\eta,\Delta_2^{max})~\mu \le \delta_1, \nonumber\\ 
& & & {\Psi}_{0}^{max}(\eta,\Delta_1^{max}) + {\Psi}_{1}^n(\eta,\Delta_2^{max})~\mu \le \delta_2. \nonumber \mytag{Robust CLF}\\
&&& A_c(x)u \le b_c(x), \nonumber \mytag{Constraints}\\
&&& u =u_{ff}(x) + (L_g L_f y(x))^{-1} \mu. \mytag{IO}
\end{align}
\HRule
The above can be represented in a similar form to \eqref{CLF_QP_form}, thus representing a quadratic program.

\subsection{Robust CBF-CLF-QP}
\label{app:Robust CBF-CLF-QP}
Note that the robust CBF condition in \eqref{robust_CBF_QP} is affine in $\mu_b$ and can be expressed as
\begin{equation} \label{eq:RobustCBF-Psi}
	\max_{\substack{||\Delta_1^b||\le \Delta^b_{1,max} \\ ||\Delta_2^b||\le \Delta^b_{2,max} }} 
	\Psi_0^b+ \Psi_1^b \mu_b \le 0
\end{equation}
%The CBF condition in our QPs takes the form:
%\begin{align}
%\label{constraints_ith}
%\Psi_0^b(x)+ \Psi_1^b(x) \mu_b \le 0
%\end{align}
where ``$b$'' refers to CBF constraint in the QP, and
\begin{align}
\Psi_0^b(x, \Delta_1^b)&:=\Delta_1^b-\frac{\gamma}{B(x)}, \nonumber\\
\Psi_1^b(x, \Delta_2^b)&:=1+\Delta_2^b,
\end{align}
where the above arises due to the time-derivative of the CBF from \eqref{eq:linearized_CBF_Uncertainty}.

Since $\Psi_0^b, \Psi_1^b$ are affine with respect to $\Delta_1^b, \Delta_2^b$, and with the assumptions on the bounds on the uncertainty in \eqref{eq:CBF_uncertainty_bound}, the robust CBF condition \eqref{eq:RobustCBF-Psi} will hold if the following two inequalities hold
\begin{align}
\Psi_{0,max}^b(x)+ \Psi_{1,p}^b(x) \mu_b \le 0, \nonumber\\
\Psi_{0,max}^b(x)+ \Psi_{1,n}^b(x) \mu_b \le 0.
\end{align}
where
\begin{align}
	\Psi_{0,max}^b&:=\Delta_{1,max}^b-\frac{\gamma}{B(x)},\\
	\Psi_{1,p}^b&:=1 + \Delta_{2,max}^b,\\
	\Psi_{1,n}^b&:=1 - \Delta_{2,max}^b.
\end{align}
%\begin{align}
%\Psi_{0,max}^b&:=max(\Psi_{0,p}^b,\Psi_{0,n}^b),\\
%\Psi_{0,p}^b&:=\Psi_0^b+ \Psi_1^b \Delta_{1,max}^b,\\
%\Psi_{0,n}^b&:=\Psi_0^b- \Psi_1^b \Delta_{1,max}^b,\\
%\Psi_{1,p}^b&:=\Psi_1^b (1 + \Delta_{2,max}^b),\\
%\Psi_{1,n}^b&:=\Psi_1^b (1 - \Delta_{2,max}^b).
%\end{align}
%
%Under the effect of uncertainty, the robust control would consider
%\begin{align}
%\tilde{\mu}_b=\mu_b+ \Delta_1^b+ \Delta_2^b \mu_b
%\end{align}
%Therefore, we should satisfy the following conditions:
%\begin{align}
%\Psi_0^b(x)+ \Psi_1^b(x) (\mu_b+ \Delta_1^b+ \Delta_2^b \mu_b) \le 0
%\end{align}
%where the uncertainties are bounded
%\begin{align}
%||\Delta_1^b|| \le \Delta_{1,max}^b,\\
%||\Delta_2^b|| \le \Delta_{2,max}^b.
%\end{align}
%
%Similar to Robust CLF-QP, we now define:
%\begin{align}
%\Psi_{0,max}^b&:=max(\Psi_{0,p}^b,\Psi_{0,n}^b),\\
%\Psi_{0,p}^b&:=\Psi_0^b+ \Psi_1^b \Delta_{1,max}^b,\\
%\Psi_{0,n}^b&:=\Psi_0^b- \Psi_1^b \Delta_{1,max}^b,\\
%\Psi_{1,p}^b&:=\Psi_1^b (1 + \Delta_{2,max}^b),\\
%\Psi_{1,n}^b&:=\Psi_1^b (1 - \Delta_{2,max}^b).
%\end{align}
%
%The robust version of the constraints \eqref{constraints_ith} will become:
%\begin{align}
%\Psi_{0,max}^b(x)+ \Psi_{1,p}^b(x) \mu_b \le 0,\\
%\Psi_{0,max}^b(x)+ \Psi_{1,n}^b(x) \mu_b \le 0.
%\end{align}
We then can incorporate the above robust CBF conditions into the robust CLF-QP \eqref{Robust_CBF_CLF_QP_form} resulting in a quadratic program.

\subsection{Robust Constraints}
\label{app:Robust Constraints}
%The same principle can be applied for robustifying constraints with
%\begin{align}
%\Psi_0^c=0; \Psi_1^c=1.
%\end{align}

Note that the robust constraints condition in \eqref{robust_CLF_QP_robust_constraint} is affine in $\mu_c$ and can be expressed as
\begin{equation} \label{eq:Robust-constraints-Psi}
	\max_{\substack{||\Delta_1^c||\le \Delta^c_{1,max} \\ ||\Delta_2^c||\le \Delta^c_{2,max} }} 
	\Psi_0^c+ \Psi_1^c \mu_c \le 0
\end{equation}
%The CBF condition in our QPs takes the form:
%\begin{align}
%\label{constraints_ith}
%\Psi_0^b(x)+ \Psi_1^b(x) \mu_b \le 0
%\end{align}
where ``$c$'' refers to constraints, and
\begin{align}
\Psi_0^c(x, \Delta_1^c)&:=\Delta_1^c, \nonumber\\
\Psi_1^c(x, \Delta_2^c)&:=1+\Delta_2^c,
\end{align}
where the above arises due to the form of the constraints in \eqref{eq:constraints-mu_c}.  The same procedure as what was done for the robust CBF in the previous section can be carried out for the robust constraints as well to show how the max problem gets converted to a set of linear inequalities and thus the min-max problem then becomes a quadratic program even for the robust constraints as well.
